# Supplementary material for: Understanding Retrieval-Augmented Task Adaptation for Vision-Language Models
Source: arXiv:2405.01468 source file (2024-05-02)
Supplement: Supplementary file 1 [file bak_appendix_12072023.tex]

\begin{center}
	\textbf{\LARGE Appendix }
\end{center}
%%%%%%%%%%%%%%%%%%%%%%%%%%%%%%%%%%%%%%%%%%%%%%%%%%%%%%%%%%%%%%%%%%%%%%%%%%%%%%%
%%%%%%%%%%%%%%%%%%%%%%%%%%%%%%%%%%%%%%%%%%%%%%%%%%%%%%%%%%%%%%%%%%%%%%%%%%%%%%%
\section{Problem Setup}  
In this section, we consider a one-shot setting for simplification. 

\paragraph{Notation.}
We denote $[n]:= \{1,2,\dots, n\}$.

\paragraph{Data.} 
We have $\nc$ number of classes and $\nk$ number of retrieved samples per class. Thus, there are $\nc\nk$ retrieved samples in total. Suppose that the hidden representation dimension is $\nd$. For each class $i \in [\nc]$, we have a text embedding $\t_i \in \R^\nd$ and one-shot image embedding $\s_i \in \R^\nd$. Let $\T = [\t_1, \dots, \t_c] \in \R^{\nd \times \nc}$ and $\S = [\s_1, \dots, \s_c] \in \R^{\nd \times \nc}$.
Let $\q \in \R^\nd$ be a query image embedding, and $\K = [\k_1, \dots, \k_{\nc\nk}] \in \R^{\nd \times \nc\nk}$ be the sorted retrieved image embedding, where $\k_i \in \R^\nd$ be the $\idx(i):=[(i-1)//\nk+1]$-th class of retrieved samples for any $i \in [\nc\nk]$. We suppose that all vectors are normalized, i.e., $\|\q\|_2 = \|\k\|_2 = \|\t\|_2 = 1$ as CLIP~\citep{radford2021learning}. 

\paragraph{Retrieved Data.}
Suppose we have a large image dataset for data retrieval and we use $R$ to denote the embedding of these images. There are two ways to retrieve data: (1) Text to Image T2I and (2) Image to Image I2I. Let $\k$ be a feature embedding in $R$. For each class $i \in [\nc]$, we retrieve the top $\nk$ similar images based on the metric (1) $\k^\top \t_i$ for T2I and (2) $\k^\top \s_i$ for I2I.  

\paragraph{Prediction.}
If we do not use the retrieved samples, we can directly use $\f_t(\q) = \T^\top \q$ to obtain a class-wise logit for zero-shot classification as CLIP. 
We can also use $\f_s(\q) = \S^\top \q$ to obtain a class-wise logit for one-shot classification without using text information. 

Now, we consider a self-linear attention model~\citep{zhang2023trained} to use the retrieved data. During classification, the class-wise logits of a query are $\f_k(\q) = \V {\K^\top \q \over \nk}$, where $\nk$ is used for normalization in self-attention. $\V \in \R^{\nc \times \nc\nk}$ is a value matrix and
\begin{itemize}
    \item $\V$ can be fixed as \citet{zhang2022tip}, where $\V_{\idx(i),i} = 1$ for any $i \in [\nc\nk]$ and all other entries being $0$ otherwise. 
    \item $\V$ can be learned parameters (TBD).
\end{itemize}

For simplicity, we first consider a fixed $\V$. Now, when we use the text embedding as \citet{udandarao2023sus}, we have $\f_2(\q) = \V {\K^\top \T \T^\top \q \over \nk}$. Let $\bK =  {\K \V^\top \over \nk} \in \R^{\nd \times \nc}$ be the average retrieved representation for each class. Then, we directly have $\f_1(\q) =  {\bK^\top \q }$ and $\f_2(\q) = {\bK^\top \T \T^\top \q }$. We can see that $f_1$ is a special case when $\T$ is an identity matrix. (TBD, we may generalize $\T^\top \q$ to element-wise $\simf(\T, \q)$).



We consider the 

\subsection{Binary classification}
For simplicity, we consider binary classification first. Let $\ell$ be the logistic loss or the hinge loss, and $y \in \{-1, +1\}$ be the label of the first and second class. Let $\k_+ = \bK_{:,1}$ and $\k_- = \bK_{:,2}$ be the average retrieved representations of the first and second classes. We also have $\T = [\t_1, \t_2]$. 

% \begin{assumption}\label{assumption:orthogonal}
%     We assume that $\t_1$ and $\t_2$ are (almost TBD) orthogonal to each other. (Each concept in CLIP is almost orthogonal with each other). 
% \end{assumption}

Let $q_i = \t_i^\top \q$, $k_{+,i} = \t_i^\top \k_+$, $k_{-,i} = \t_i^\top \k_-$ for $i \in \{1,2\}$. We have the loss
\begin{align}
    \cL(\f_2, (\q, y)) = & \ell\left( y(\k_+^\top \T \T^\top \q - \k_-^\top \T \T^\top \q)\right) \\
     = & \ell\left( y(\k_+ - \k_-)^\top [\t_1, \t_2] [\t_1, \t_2]^\top \q\right) \\
     = & \ell\left( y ((k_{+,1} - k_{-,1}) q_1 - (k_{-,2} - k_{+,2}) q_2)\right).
\end{align}

Note that if $ y (q_1 - q_2) > 0$, then the model $\f_0$ can resolve the classification directly without using the retrieved images.     
Now, we are more interested in the case when $ y (q_1 - q_2) < 0$. 



Using the intuition of~\cite{chen2023understanding}, we define a CLIP similarity metric $\alpha, \gamma$ such that with probability at least $1-\alpha$, we have 

\subsection{Muti-class classification}

\newpage

\subsection{TODO}
\begin{itemize}
    \item Tip-adapter
    \item  I2I is better than T2I
    \item ensemble is better than zero-shot, binary 2 cases, and multiclass 3 cases.  
    \item label noises. 
    \item Top3 ACC $->$ true logits are large but not max. 
\end{itemize}


% \subsection{Some thoughts}
% \begin{itemize}
%     \item Make assumptions directly on the representation.
%     \item Linear data linear model
%     \item consider language and image graph. Connection image and caption ...
% \end{itemize}



% \subsection{TODO}
% $y$ can be seen as $\z$ in Quanquan's paper. Three gap (1) $\q$ and $\t$; $\k$ and $\t$
% (2) $\q$ and $\k$, (3) $\q, \k$ and $y$, (4) $\t$ and $y$. 

% \begin{itemize}
%     \item Use Quanquan's data model + Pretraining results. 
%     $\z, \bxi$. $\x_q \sim T_1(\z, \bxi_1)$, $\x_k \sim T_1(\z, \bxi_2)$, $ \y \sim T_2(\z, \bzeta)$. 
%     \item $\t = h(\y), \q = g(\x_q), \k = g(\x_k)$. 
%     \item By Quanquan's paper, we have 
%     \item Make assumption on representation. 
% \end{itemize}

% f(xq,xk) 

% f(xq,y), f(xk,y)

% Ultimate goal: zoclip error - optimal error $<$ fraction of label noise (mismatched label)  + retrieved sample size + retrieval method (I2I, T2I) $<$ covariate shift 

% zoclip error - optimal error $<$ retrieved sample size + retrieval method (I2I, T2I) $<-$ covariate shift 
